# Supplementary material for: Secure Generalization through Stochastic Bidirectional Parameter Updates Using Dual-Gradient Mechanism
Source: arXiv:2504.02213 source file (2025-04-03)
Supplement: Supplementary file 1 [file X_suppl.tex]

\clearpage
\setcounter{page}{1}
% \setcounter{section}{0} 
% Sets the section counter to start from 1 (or any number you choose)

\maketitlesupplementary

% **************************************

\section{Convergence Analysis}
Our global model is aggregated from all the trained local models similar to FedAvg. Let $t$ denote the $t^{th}$ SGD iteration on the local client, and each local client undergoes $E$ SGD training iterations, $w_{glb}$ denotes the aggregated model. For $i = 1, 2, \dots, K$, our method satisfies the following property:
\begin{equation}\label{eq_sup_1}
\alpha^2 \|{w}_{{glb}}^n - {w}_{{glb}}^{n-1}\|^2 \le  \|{w}_{{i,n}}^{loc} - {w}_{{glb}}^{n}\|^2 \le 4\alpha^2 \|{w}_{{glb}}^{n} - {w}_{{glb}}^{n-1}\|^2 
\end{equation}
where $\mathbf{w}_{i,n}^{{loc}}$ denotes the $i^{th}$ mutated weights in the $n^{th}$ round. Inspired by~\cite{li2019convergence}, the following assumptions on the loss functions of local clients (i.e., $f_1, f_2, \dots, f_K$) can be considered.\\
\textbf{Assumption 1:} For $i \in \{1, 2, \dots, K\}$, $f_i$ is $L$-smooth, where $f_i(v) \leq f_i(w) + (v - w)^T \nabla f_i(w) + \frac{L}{2} \|v - w\|_2^2$.\\
\textbf{Assumption 2:} For $i \in \{1, 2, \dots, K\}$, $f_i$ is $\mu$-strongly convex, where $f_i(v) \geq f_i(w) + (v - w)^T \nabla f_i(w) + \frac{\mu}{2} \|v - w\|_2^2$.\\
\textbf{Assumption 3:} The variance of stochastic gradients is bounded by $\sigma_i^2$, i.e., $\mathbb{E}\|\nabla f_i(w; \xi) - \nabla f_i(w)\|^2 \leq \sigma_i^2$, where $\xi$ is a data batch of the $i^{th}$ client in the $t^{th}$ FL round.\\
\textbf{Assumption 4:} The expected squared norm of stochastic gradients is bounded by $G^2$, i.e., $\mathbb{E}\|\nabla f_i(w; \xi)\|^2 \leq G^2$.\\
Based on these assumptions, our convergence can be obtained as:\\
\textbf{Theorem 1. (Convergence of SBPU)} Let Assumption 1-4 hold. If there are $n$ FL rounds during the FL training process. Let $T = n \times E$ denotes total number of SGD iterations and $\eta_t = \frac{2}{\mu (t + \gamma)}$ is learning rate. Let $\kappa = \frac{L}{\mu}$, $\gamma = \max(8\kappa, E)$. We have
\begin{equation}
\mathbb{E}[f({w}_T) - f^*] \leq \frac{4 \kappa}{\gamma + T} (\frac{B}{2\mu} + L \|{w}_1 - {w}^*\|^2)\notag{}
\end{equation}
where $B = \frac{1}{K^2} \sum_{i=1}^K \sigma_i^2 + \frac{32 \alpha^2}{1-4\alpha^2}(E - 1)^2 G^2$.\\ 
\noindent
% Theorem 1 computes loss for SBPU between $f^*$ (optimal weight) and $f({w}_T)$ in the $T^{th}$ interaction and indicates a convergence rate similar to FedAvg (detailed in~\cite{li2019convergence}).\\
\noindent
\textbf{Proof:}
Our methodology (SBPU) follows a convergence criteria similar to~\cite{li2019convergence} with minor modifications to Lemma (3). Therefore, we only focus on the modification involved in Bounding the divergence of $w_t^k$. Since SBPU requires a communication each $E$ steps. Therefore, for any $t \geq 0$, there exists a $t_0 \leq t$, such that $t - t_0 \leq E - 1$ and $\mathbf{w}_{t_0}^k = \overline{\mathbf{w}}_{t_0}$ for all $k = 1, 2, \cdots, N$. Also, we use the fact that $\eta_t$ is non-increasing and $\eta_{t_0} \leq 2\eta_t$ for all $t - t_0 \leq E - 1$, then
using Lemma (3)~\cite{li2019convergence} and Eq.~\ref{eq_sup_1}:

\begin{align*}
& \mathbb{E} \sum_{k=1}^N p_k \left\| \overline{\mathbf{w}}_t - \mathbf{w}_t^k \right\|^2 \\
&\leq \mathbb{E} \sum_{k=1}^N p_k ~4 \alpha^2 \left\| \left( \mathbf{w}_t^k - \overline{\mathbf{w}}_{t-1} \right) - \left( \mathbf{w}_t^k - \overline{\mathbf{w}}_{t} \right) \right\|^2 \\
&\leq \mathbb{E} \sum_{k=1}^N p_k \big( 4 \alpha^2 \left\| \mathbf{w}_t^k - \overline{\mathbf{w}}_{t-1} \right\|^2 
    + 4 \alpha^2 \left\| \mathbf{w}_t^k - \overline{\mathbf{w}}_{t} \right\|^2 \big) \\
&\quad \text{(since } \|a+b\|^2 \leq \|a\|^2 + \|b\|^2, \text{ where } a \text{ and } b \text{ are vectors)} \\
&\leq \mathbb{E} \sum_{k=1}^N p_k 4 \alpha^2 \left\| \mathbf{w}_t^k - \overline{\mathbf{w}}_{t-1} \right\|^2 
    + \mathbb{E} \sum_{k=1}^N p_k 4 \alpha^2 \left\| \overline{\mathbf{w}}_{t} - \mathbf{w}_t^k \right\|^2 \\
&\leq \frac{4 \alpha^2}{1 - 4 \alpha^2} \mathbb{E} \sum_{k=1}^N p_k \left\| \mathbf{w}_t^k - \overline{\mathbf{w}}_{t-1} \right\|^2 \\
&\leq \left( \frac{4 \alpha^2}{1 - 4 \alpha^2} \right) \sum_{k=1}^N p_k \mathbb{E} \sum_{t=t_0}^{t-1} (E-1) \eta_t^2 \left\| \nabla F_k(\mathbf{w}_t^k, \xi_t^k) \right\|^2 \\
&\leq \left( \frac{4 \alpha^2}{1 - 4 \alpha^2} \right) \sum_{k=1}^N p_k \sum_{t=t_0}^{t-1} (E-1) \eta_{t_0}^2 G^2 \\
&\leq \left( \frac{4 \alpha^2}{1 - 4 \alpha^2} \right) \sum_{k=1}^N p_k \eta_{t_0}^2 (E-1)^2 G^2 \\
&\leq \left( \frac{4 \alpha^2}{1 - 4 \alpha^2} \right) 4 \eta_t^2 (E-1)^2 G^2 \\
&\leq \frac{16 \alpha^2 \eta_t^2}{1 - 4 \alpha^2} (E-1)^2 G^2.
\end{align*}

Our first inequality follows $\mathbb{E}[\|X - \mathbb{E}[X]\|^2] \leq \mathbb{E}[\|X\|^2]$ where $X = \mathbf{w}_t^k - \overline{\mathbf{w}}_{t_0}$ with probability $p_k$. We use Jensen's inequality in the second inequality, which gives:
\begin{align*}
\|\mathbf{w}_t^k - \overline{\mathbf{w}}_{t_0}\|^2 = \left\|\sum_{t=t_0}^{t-1} \eta_t \nabla F_k(\mathbf{w}_t^k, \xi_t^k) \right\|^2 \\
\leq (t - t_0) \sum_{t=t_0}^{t-1} \eta_t^2 \| \nabla F_k(\mathbf{w}_t^k, \xi_t^k) \|^2.
\end{align*}
In the third inequality, we use $\eta_t \leq \eta_{t_0}$ for $t \geq t_0$ and $\mathbb{E}[\| \nabla F_k(\mathbf{w}_t^k, \xi_t^k) \|^2] \leq G^2$ for $k = 1, 2, \dots, N$ and $t \geq 1$. We use $\eta_{t_0} \leq 2 \eta_{t_0 + E} \leq 2 \eta_t$ for $t_0 \leq t \leq t_0 + E$ in the last inequality.\\

Following Lemma (1), (2), and (3) from~\cite{li2019convergence}, we get:\\
\begin{equation}
\mathbb{E}[f({w}_T) - f^*] \leq \frac{4 \kappa}{\gamma + T} (\frac{B}{2\mu} + L \|{w}_1 - {w}^*\|^2)\notag{}
\end{equation}
where $B = \frac{1}{K^2} \sum_{i=1}^K \sigma_i^2 + \frac{32 \alpha^2}{1-4\alpha^2}(E - 1)^2 G^2$. For additional details, please refer to~\cite {li2019convergence}.

\section{Classification Results:}
We select a random user to test accuracy since our approach doesn't have a global classification model. We provide the highest classification accuracy obtained by our model and compare it with different techniques in Table~\ref{tab:classification_accuracy_mnist_fmnist}. Our method surpassed the available techniques and obtained the highest classification accuracy for all the datasets. 

\begin{table}[h]
\centering
\begin{tabular}{ccc}
\hline
\textbf{Method} & \textbf{MNIST} & \textbf{FMNIST} \\ \hline
ATS    & 98.96 & 89.23 \\ 
EtC    & 98.06 & 89.41 \\ 
DP1    & 97.42 & 85.58 \\ 
DP2    & 97.54 & 85.01 \\ 
GC1    & 97.61 & 85.81 \\ 
GC2    & 97.22 & 85.09 \\ 
FedCG  & 98.6  & 88    \\ 
PPIDSG & 99.43 & 91.6  \\ \hline
\textbf{\textit{Ours}}   & \textbf{\textit{99.54}} & \textbf{\textit{92.14}} \\ \hline
\end{tabular}
\caption{Classification accuracy obtained for different policies. Here, DP1: DP$<$5,10$>$, DP2: DP$<$20,5$>$, GC1: GC (10\%), GC2: GC (40\%).} \label{tab:classification_accuracy_mnist_fmnist}
\end{table}

\section{Defense Accuracy Under Different Settings:}
In Fig.~\ref{fig:compare_sota_setting_plot}, we also compared the defense accuracy of our approach with SOTA settings: 1) Original Image; 2) No update. Original Image (benchmark) represents the original image as inputs to $F$, which jointly trains with $C$; no update denotes the setting that does not train the classifier and only uses the initial parameters. We observe that our approach surpasses no update and is slightly lower than the Original Image. It is important to note that our method does not use the original image input and does not share the classifier model parameters.\\

\begin{figure}[h]
    \centering
    \includegraphics[width=9cm, height=7cm]{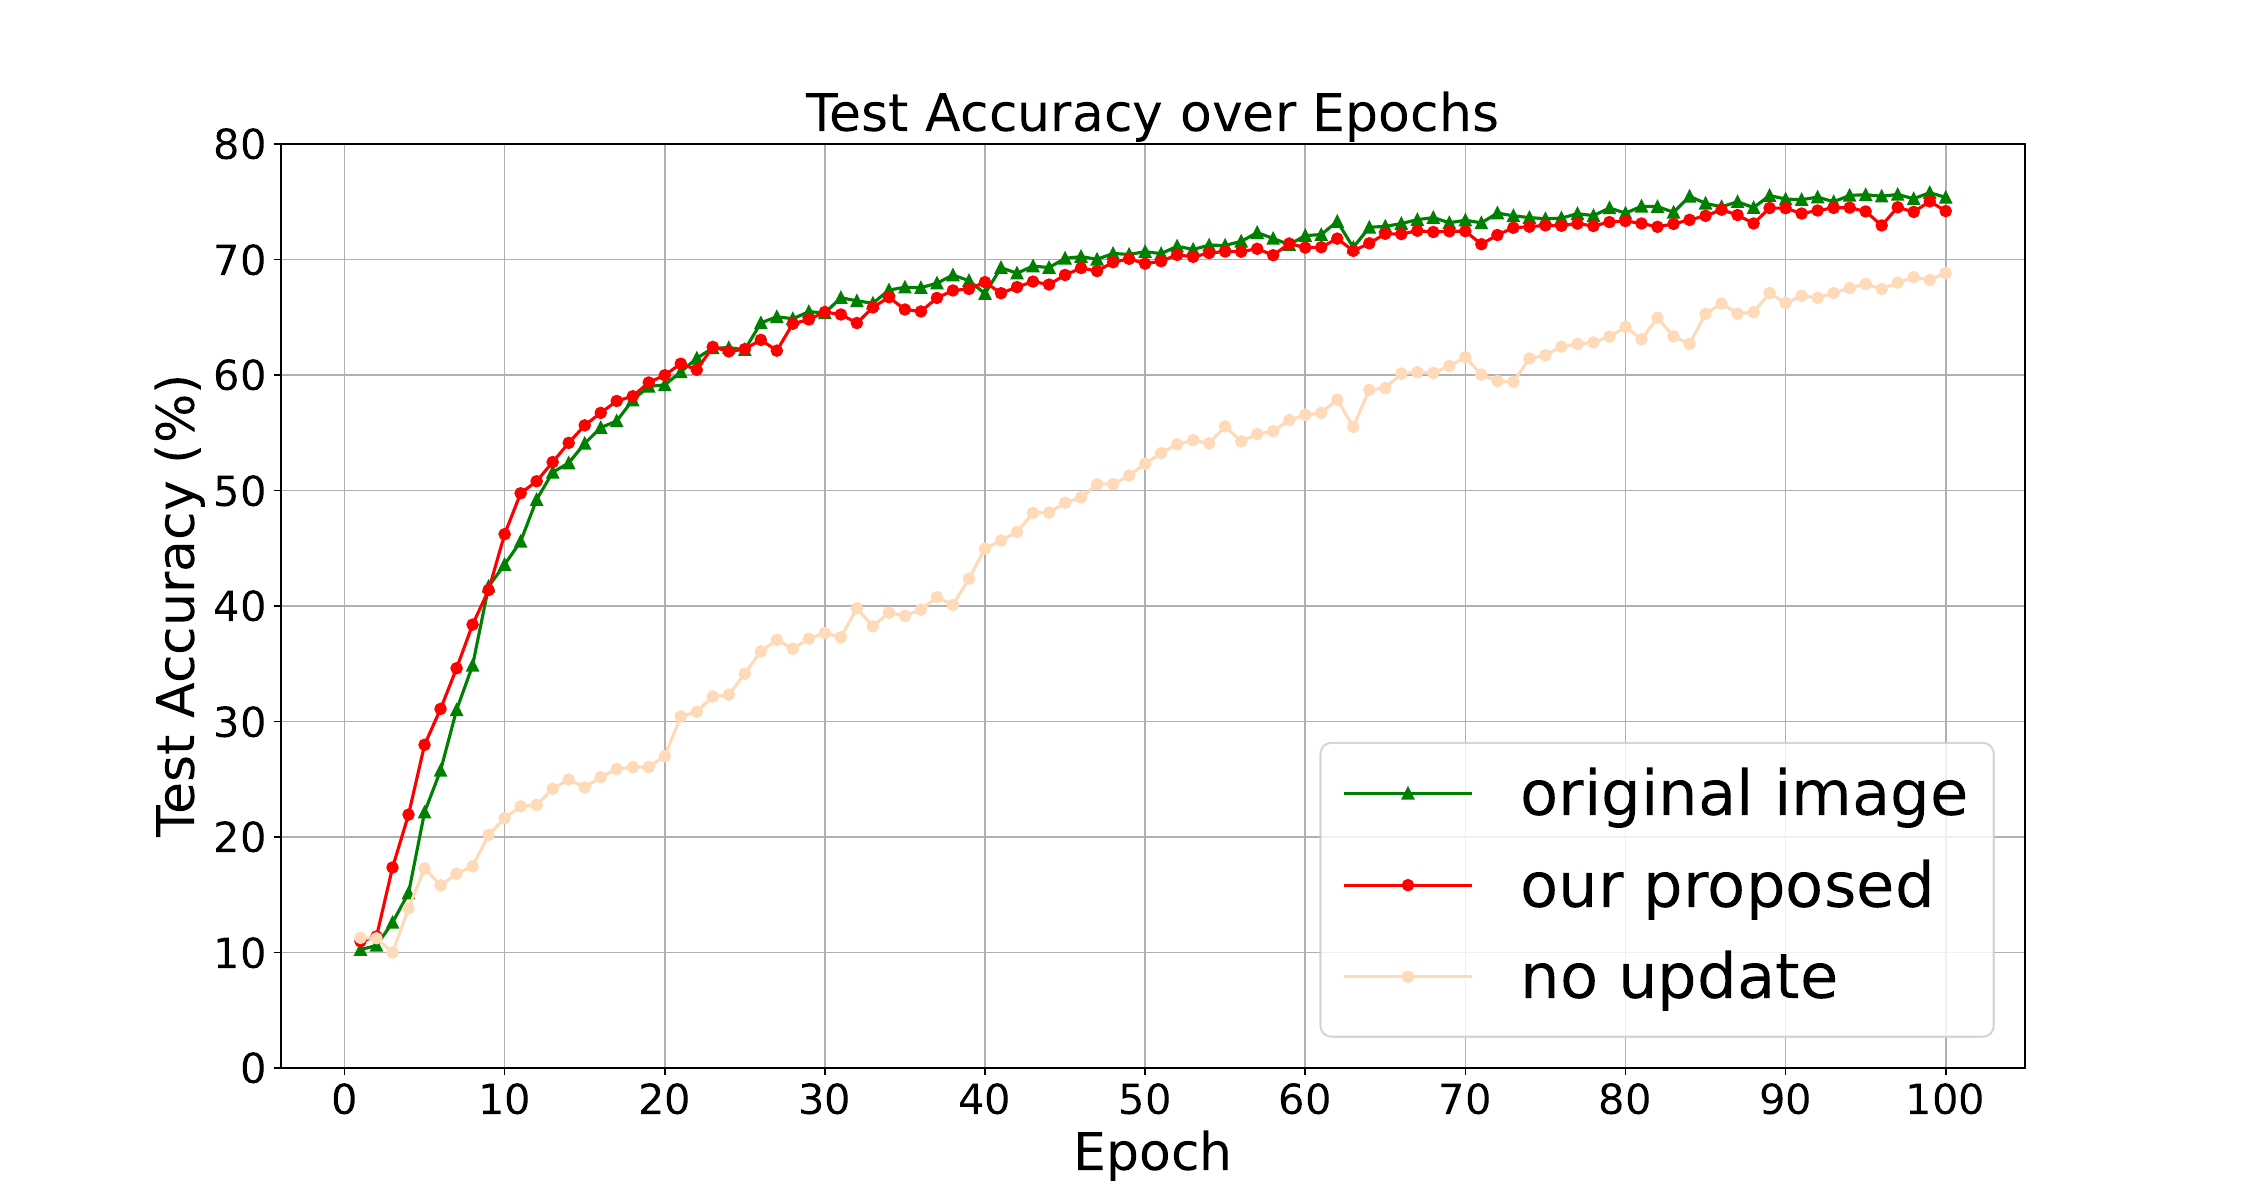}
    \caption{Comparison of defense accuracy of the proposed approach using CIFAR10 dataset under different settings: 1) using ``original image''; 2) using ``no update''. }
    \label{fig:compare_sota_setting_plot}
\end{figure}

\section{Ablation Experiment on Block Size and Number of Clients:}
We also analyze the effect of block size used during image encryption and the number of clients in FL on defense accuracy in Fig.~\ref{fig:block_size} and Fig.~\ref{fig:clients}. We observe that the block size during image encryption does not make significant changes to model performance. When we increased the number of clients, we observed that the proposed method consistently outperformed PPIDSG, which validates the practical utility and robustness of our model.

\begin{figure}[h]
\centering
    \includegraphics[width=7.8cm, height=3.3cm]{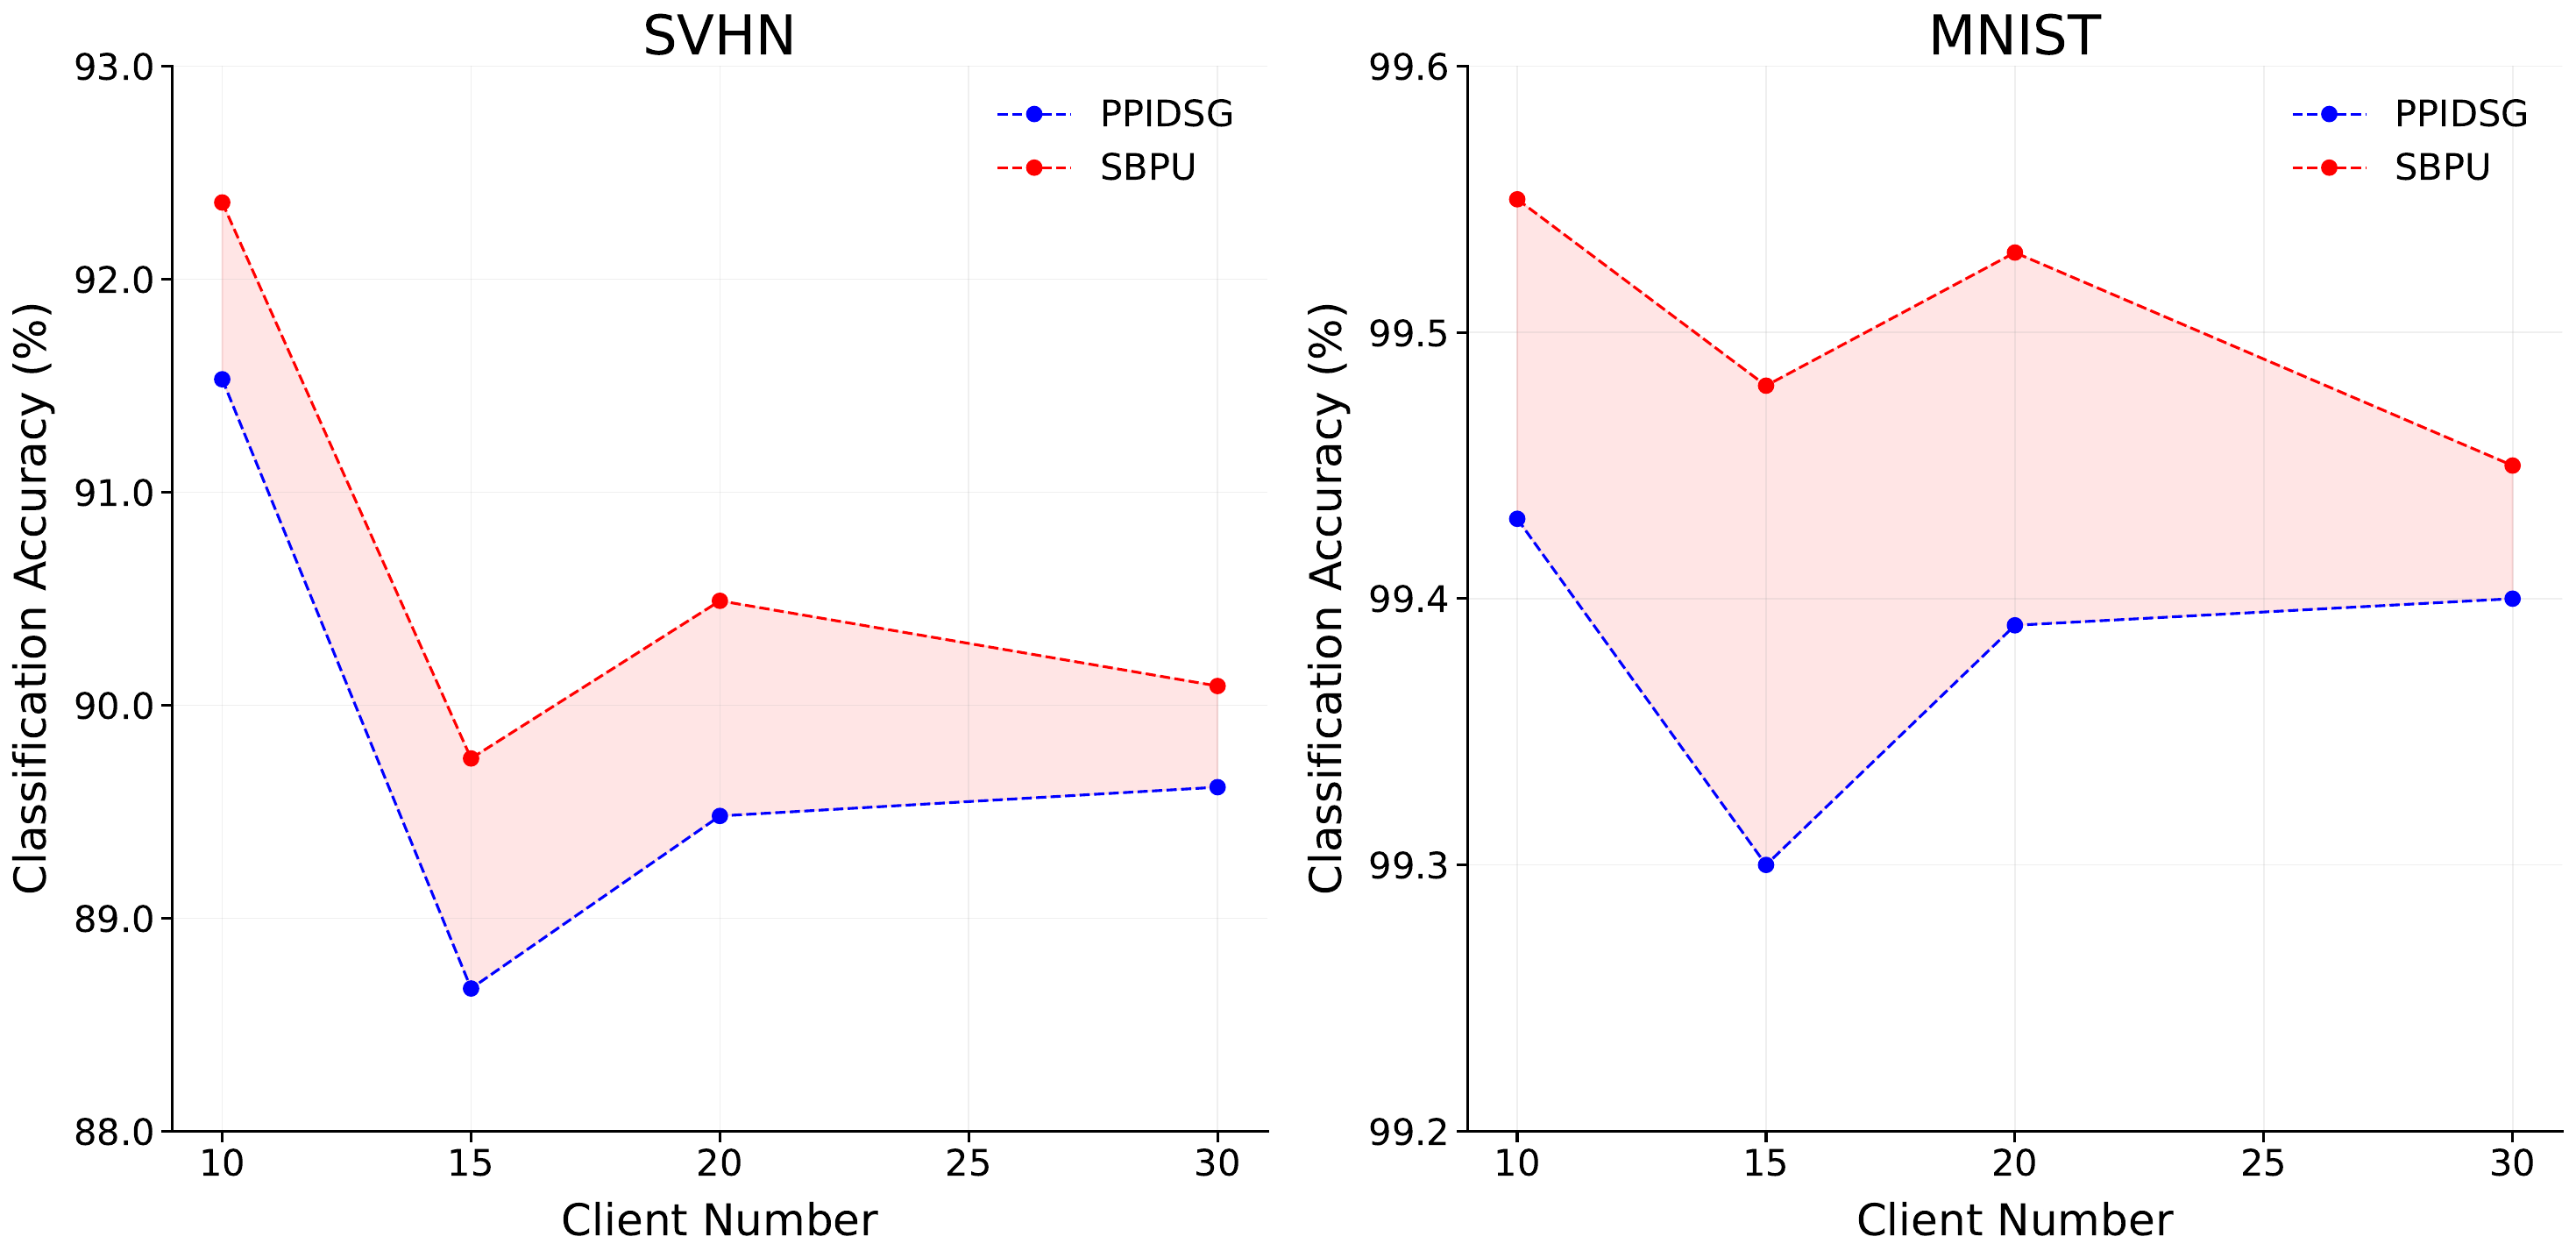}
    \caption{Comparative analysis of the effect of increasing client numbers on PPIDSG and the proposed method (SBPU) over SVHN and MNIST datasets.}\label{fig:block_size}
\end{figure}

\begin{figure}[h]
    \centering
    \includegraphics[width=9.3cm, height=6cm]{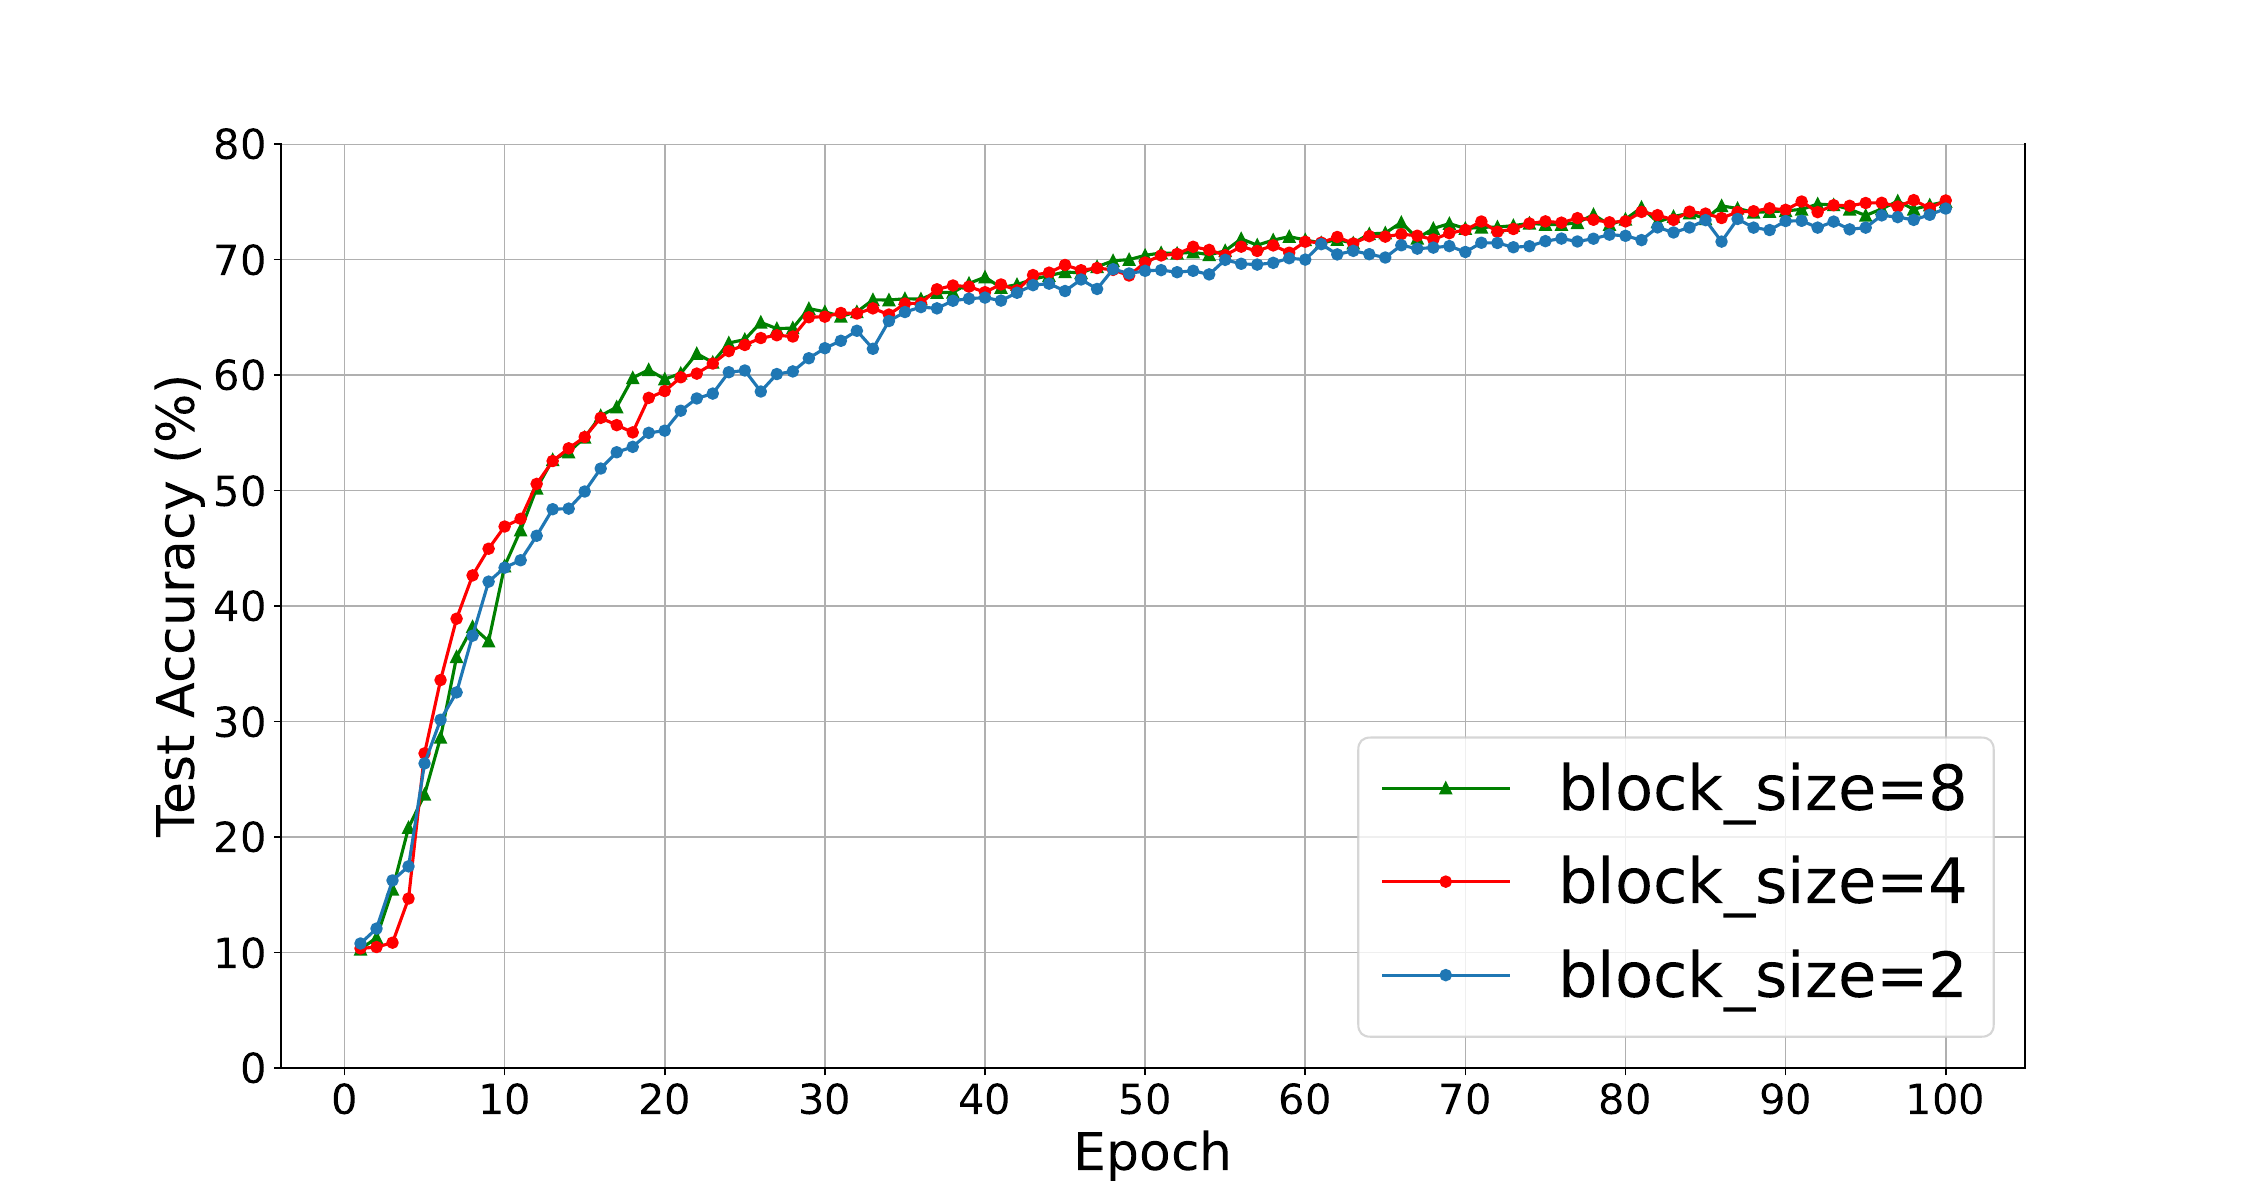}
    \caption{Effect of varying block size in image encryption algorithm on the proposed approach.}\label{fig:clients}
\end{figure}

\section{Histogram Visualization Against Image Reconstruction (IR) Attack:}
In Fig.~\ref{fig:SVHN_ORIGINAL_SUPPLY} and Fig.~\ref{fig:SVHN_GENERATED_SUPPLY}, we visualize the original \& reconstructed image through a histogram distribution plot. We can observe that the original image provides the histogram distribution as per visual information present in the image, while the generated image using our approach does not provide visual cues related to the original image and provides uniform distribution in the histogram (i.e., resist privacy leakage). The slight peaks at the end of the histogram are due to the blank areas present in the generated image.

\section{Hyperparameter Tuning for Diversity Rate:}
We experimented with different values for Hyperparameter Tuning for Diversity Rate ($\beta$) for different datasets, i.e., MNIST, FMNIST, CIFAR10, and SVHN, in Table~\ref{tab:beta_tuning_supply}.

\begin{table}[h]
    \centering
    
    % \fontsize{7}{12}\selectfont
\begin{tabular}{c c c cc }
\hline
\textbf{Datasets} & \textbf{$\beta$}& \textbf{Precision} & \textbf{Recall} & \textbf{F1-Score}  \\
\hline
\multirow{4}{*}{MNIST} & \textbf{0.025} & \textbf{0.10(0.90)} & \textbf{0.80(0.20)} & \textbf{0.18(0.33)}  \\ 
 & 0.1 & 0.10(0.90) & 0.40(0.60) & 0.16(0.72)  \\ 
 & 0.65 & 0.10(0.90) & 0.68(0.31) & 0.17(0.46)  \\ 
 & 1 & 0.09(0.87) & 0.62(0.29) & 0.16(0.44)  \\ \hline
\multirow{4}{*}{FMNIST} & \textbf{0.25} & \textbf{0.09(0.87)} & \textbf{0.60(0.30)} & \textbf{0.15(0.45)} \\ 
 & 0.35 & 0.10(0.90) & 0.61(0.40) & 0.17(0.56)  \\ 
 & 0.85 & 0.13(0.91) & 0.40(0.70) & 0.10(0.79)  \\ 
 & 1.15 & 0.10(0.90) & 0.58(0.40) & 0.17(0.55)  \\ \hline
 \multirow{4}{*}{CIFAR10} & \textbf{0.15} & \textbf{0.10(0.90)} & \textbf{0.62(0.38)} & \textbf{0.17(0.54)}  \\
 & 0.5 & 0.10(0.89) & 0.54(0.44) & 0.16(0.59)  \\ 
 & 1 & 0.12(0.92) & 0.51(0.59) & 0.19(0.71)  \\ 
& 1.5 & 0.09(0.89) & 0.42(0.53) & 0.15(0.67) \\ \hline
\multirow{4}{*}{SVHN} & 0.15 & 0.11(0.92) & 0.69(0.40) & 0.20(0.56)  \\
 & 0.55 & 0.11(0.91) & 0.72(0.34) & 0.19(0.49) \\ 
 & 1 & 0.12(0.93) & 0.70(0.41) & 0.20(0.57)  \\ 
 & \textbf{1.1} & \textbf{0.09(0.89)} & \textbf{0.58(0.37)} & \textbf{0.16(0.53)} \\
 \hline
\end{tabular}
\caption{Hyperparameter tuning for $\beta$ to decide the optimal diversity rate for the proposed approach. Here, bold entries denote the robustness of the MIA attack (less value denotes more robustness towards attack) under the All setting. The numbers in brackets represent data from non-members, while those outside parentheses represent member data.}
    \label{tab:beta_tuning_supply}
\end{table}

\begin{figure}[H]
    \centering
    \includegraphics[width=8cm, height=4.5cm]{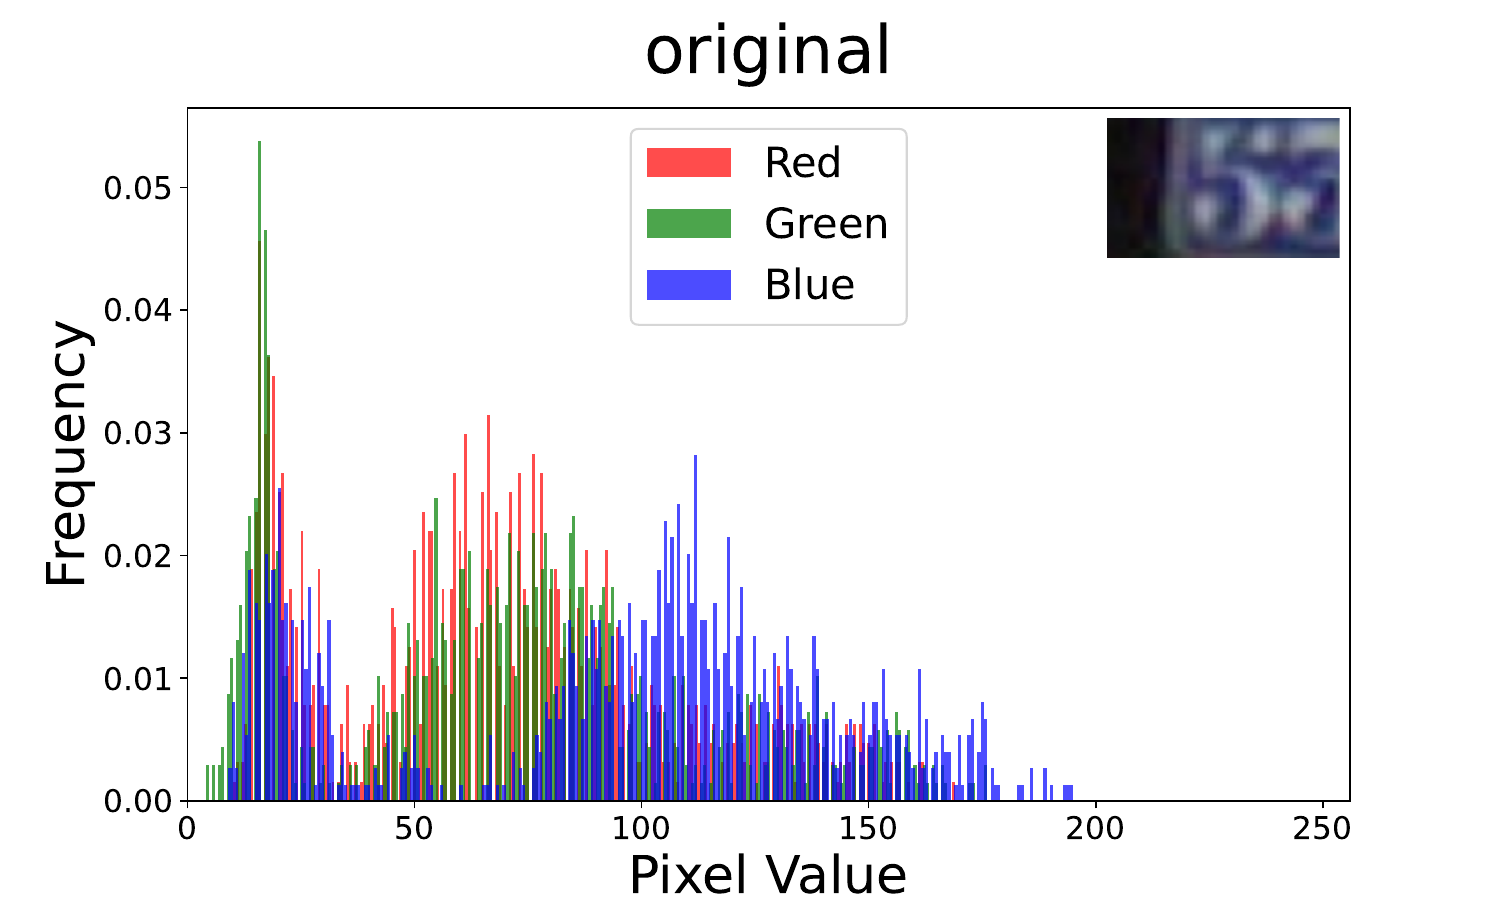}
    \caption{We visualize the pixel value distribution for an original input image from the SVHN dataset through a histogram plot. The obtained histogram distribution can provide the visual cue for the given input image for privacy leakage.} \label{fig:SVHN_ORIGINAL_SUPPLY}
\end{figure}

\begin{figure}[H]
    \centering
    \includegraphics[width=8cm, height=4.5cm]{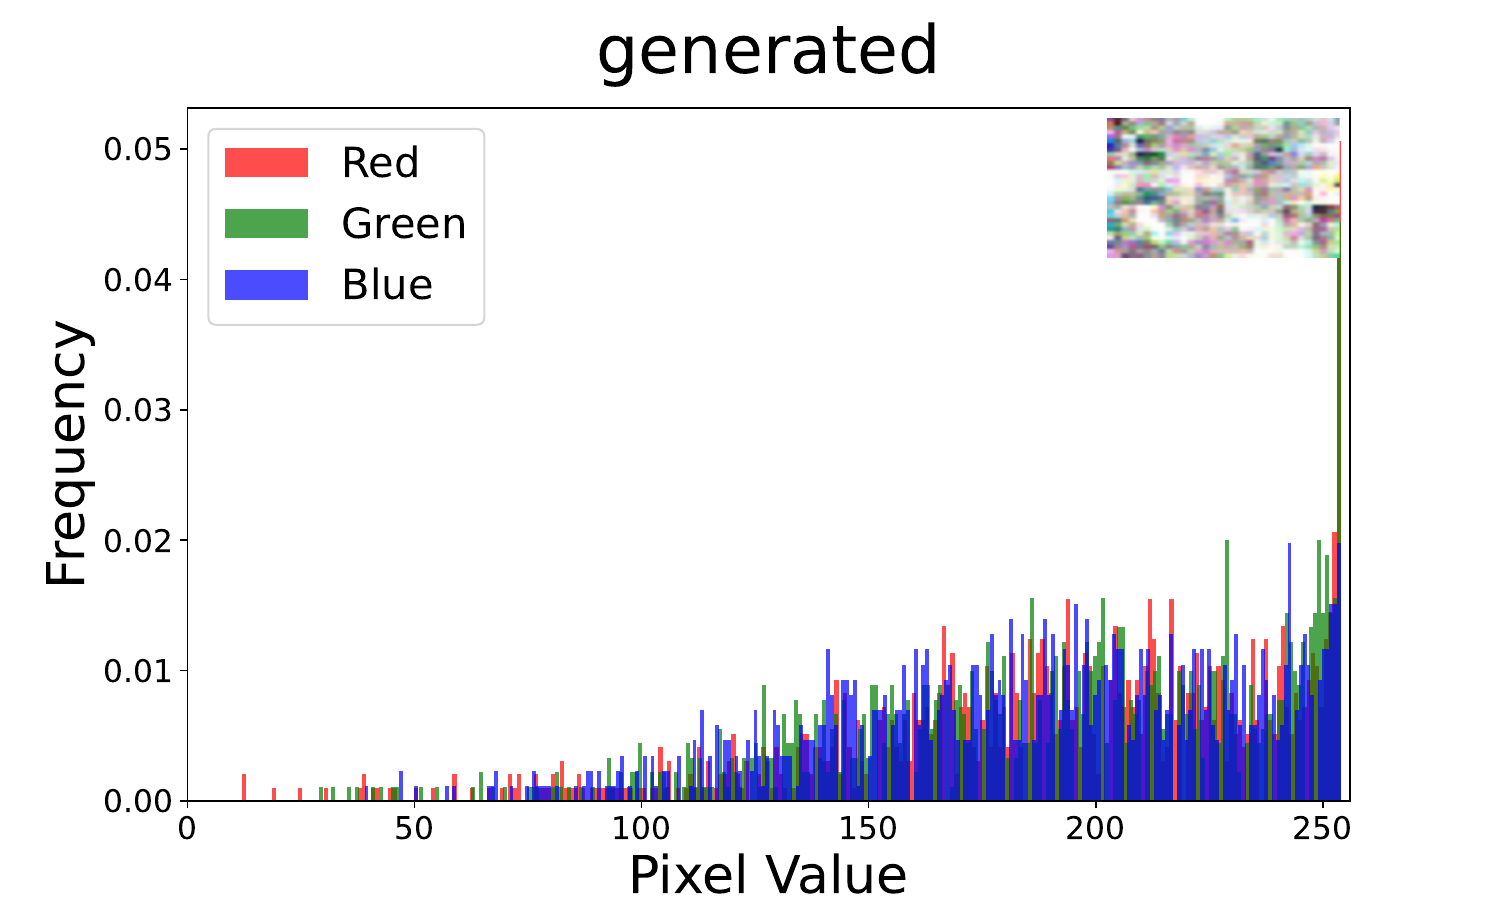}
    \caption{We visualize the pixel value distribution for the reconstructed image from the SVHN dataset obtained by the image reconstruction (IR) attack. Through histogram, we observe the uniform frequency distribution for pixel values present in the generated image, which makes our model robust against IR attack. Moreover, we can see that the reconstructed image is noisy, i.e., it does not offer visual cues for privacy leakage.} \label{fig:SVHN_GENERATED_SUPPLY}
\end{figure}

\section{Effect of Label Inference Attack (LIA):}
We provided the effect of LIA under various policies with LeNet architecture on the CIFAR10 dataset using different activation functions in Table~\ref{tab:LIA_2}. The performance of LIA under various architecture and activation functions for various datasets is shown in Table~\ref{tab:LIA_1}. We can observe that for Sigmoid activation, ATS and EtC defense mechanisms fail to resist attack irrespective of architecture type (simpler to complex design). Its primary reason is that the Sigmoid provides positive results, and hence, the attacker can perform inference effectively from the penultimate layer when the classifier is shared. For other activation functions (ReLU or LReLU) also, the LIA is successful in the range of 60.94\% to 98.44\%. For ConvNet, there is a reduction in LIA accuracy due to the MaxPool layer. We do not share the classifier parameters, so our method is resistant to LIA.

\begin{table}
\centering
        \begin{tabular}{cccccc}
            \hline
            \textbf{Methods} & \textbf{DP1} & \textbf{DP2} & \textbf{GC1} & \textbf{GC2} & \textbf{FedCG} \\
            \hline
            Sigmoid & 100 & 100 & 100 & 100 & 100 \\
            ReLU & 90.63 & 92.19 & 89.06 & 90.63 & 82.81 \\
            LReLU & 92.19 & 93.75 & 93.75 & 93.75 & 84.37 \\
            \hline
        \end{tabular}
         \caption{Performance of different policies with LeNet on CIFAR10 dataset under Label Inference Attack (LIA). We denote the different methods with their settings as DP1: DP$<$5,10$>$,
DP2: DP$<$20,5$>$, GC1: GC (10\%), GC2: GC (40\%).}
        \label{tab:LIA_2}
\end{table}

\begin{table*}
    \centering
    \begin{tabular}{ccccccccccc}
        \midrule
        \multirow{2}{*}{\textbf{Policy}} &\multirow{2}{*}{\textbf{DataSet}} & \multicolumn{3}{c}{\textbf{ResNet18}} & \multicolumn{3}{c}{\textbf{LeNet}} & \multicolumn{3}{c}{\textbf{ConvNet}} \\
        \cmidrule{3-11}
        & & Sigmoid & ReLU & LReLU & Sigmoid & ReLU & LReLU & Sigmoid & ReLU & LReLU \\
        
        \midrule
        \multirow{4}{*}{ATS} & MNIST & 100 & 98.44 & 96.88 & 100 & 98.44 & 100 & 98.44 & 76.69 & 70.31 \\
        & FMNIST & 100 & 95.31 & 95.31 & 100 & 96.88 & 98.44 & 98.44 & 73.44 & 71.88 \\
        & CIFAR10 & 100 & 93.75 & 98.44 & 100 & 92.19 & 92.19 & 95.31 & 62.5 & 60.94 \\
        & SVHN & 100 & 98.44 & 100 & 100 & 93.75 & 93.75 & 95.31 & 70.31 & 71.88 \\
        \midrule
        \multirow{4}{*}{EtC} & MNIST & 100 & 100 & 100 & 100 & 95.31 & 93.75 & 93.75 & 98.44 & 96.88 \\
        & FMNIST & 100 & 96.88 & 96.88 & 100 & 96.88 & 96.88 & 100 & 95.31 & 92.19 \\
        & CIFAR10 & 100 & 96.88 & 96.88 & 100 & 96.88 & 96.88 & 100 & 92.19 & 85.94 \\
        & SVHN & 100 & 93.75 & 95.31 & 100 & 96.88 & 96.88 & 100 & 85.94 & 87.5 \\
        \midrule
    \end{tabular}
     \caption{Performance of different policies on various datasets using different network architectures and activation functions for LIA.}
    \label{tab:LIA_1}
\end{table*}

\section{Effect of Membership Inference Attack (MIA):}%\vspace{-0.5cm}
During MIA, the test datasets are taken as shadow datasets. The network ($M_{attack}$) consists of layers with sizes 10, 128, and 2 (output layer with member, non-member classification); Adam is used as an optimizer, and the model is trained for 100 epochs with a learning rate of 0.005. We provided the comparative analysis of the proposed approach against MIA for MNIST, FMNIST, CIFAR10, and SVHN datasets in Table~\ref{tab:MIA_MNIST}, Table~\ref{tab:MIA_FMNIST}, Table~\ref{tab:MIA_CIFAR10_supplymentry}, and Table~\ref{tab:MIA_SVHN}, respectively. We also provide the defense accuracy comparison of our approach with the other defense strategies in Fig.~\ref{fig:DEFENSE_MIA_MNIST}, Fig.~\ref{fig:DEFENSE_MIA_FMNIST}, Fig.~\ref{fig:DEFENSE_MIA_CIFAR}, and Fig.~\ref{fig:DEFENSE_MIA_SVHN} under the consideration that the attacker has access to the suspect dataset, which contains images from the victim and another user (Part) or other users (All). We denote DP1, DP2, DP3, DP4, DP5, GC1, GC2, and GC3 represent DP$<$5,10$>$, DP$<$10,10$>$, DP$<$20,10$>$, DP$<$20,5$>$, DP$<$20,20$>$, GC(10\%),
GC(20\%), and GC(40\%). We observe that our method resists the attack significantly, comparing the existing defense mechanisms. The lower attack accuracy in PPIDSG is due to not sharing the classifier model parameters, while in EtC, the lower attack accuracy is due to using encrypted images. The proposed approach yields the best results.\vspace{2cm}

% \vspace{-0.5cm}
\begin{figure}
    \centering
    \includegraphics[width=8.75cm, height=4cm]{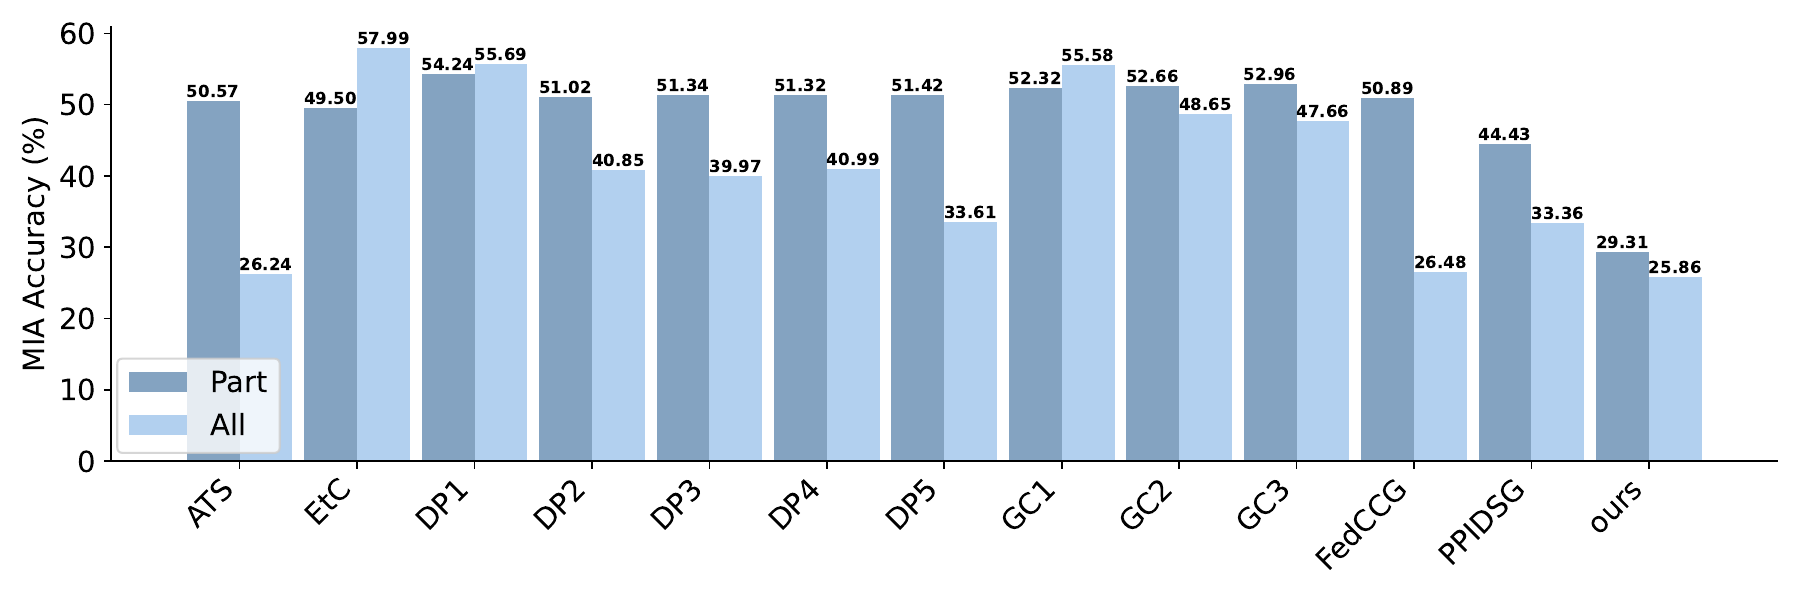}
    \caption{The MIA accuracy (\%) of different defense policies on MNIST dataset (lower is better).}\label{fig:DEFENSE_MIA_MNIST}
\end{figure}%\vspace{-1cm}

\begin{figure}
    \centering
    \includegraphics[width=8.75cm, height=4cm]{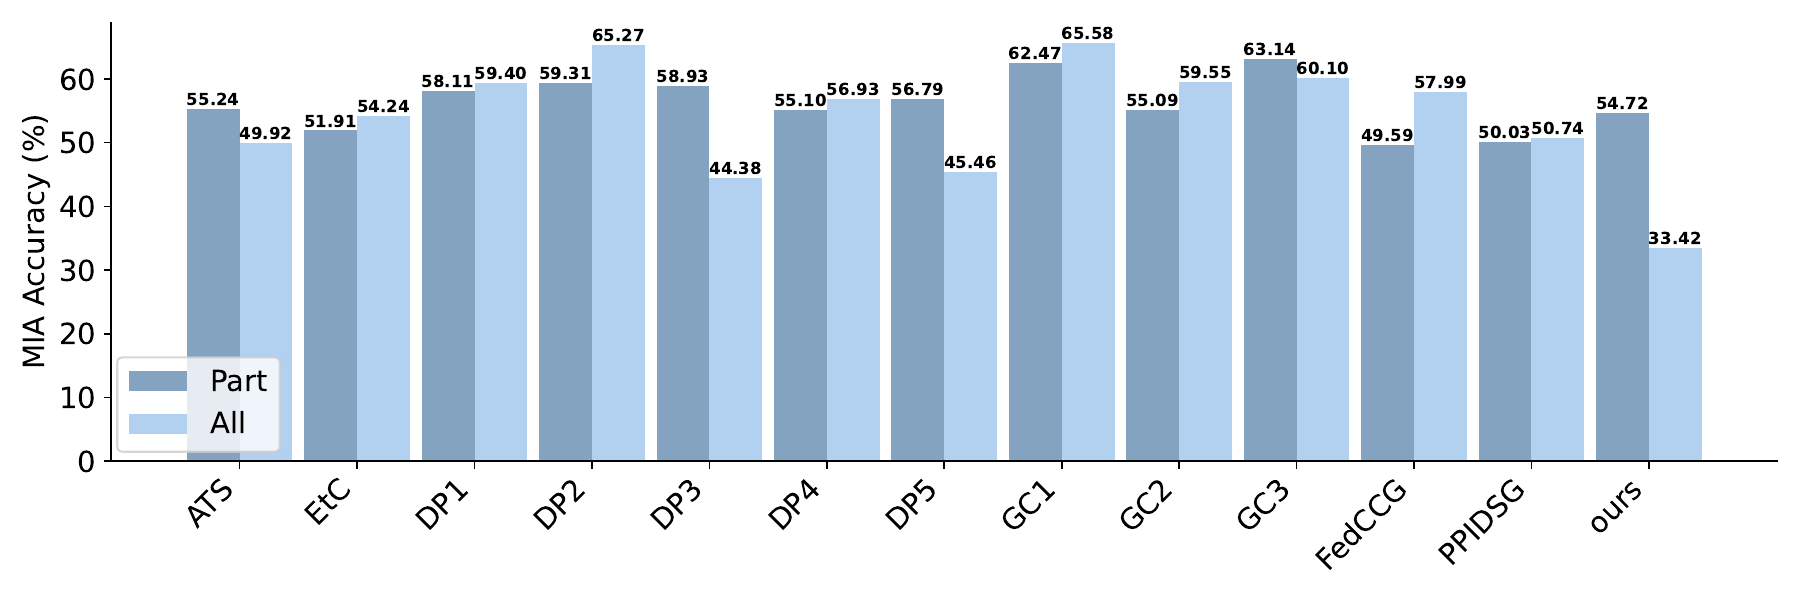}
    \caption{The MIA accuracy (\%) of different defense policies on FMNIST dataset (lower is better).}
    \label{fig:DEFENSE_MIA_FMNIST}
\end{figure}
% \vspace{-1cm}

\begin{figure}
    \centering
    \includegraphics[width=8.75cm, height=4cm]{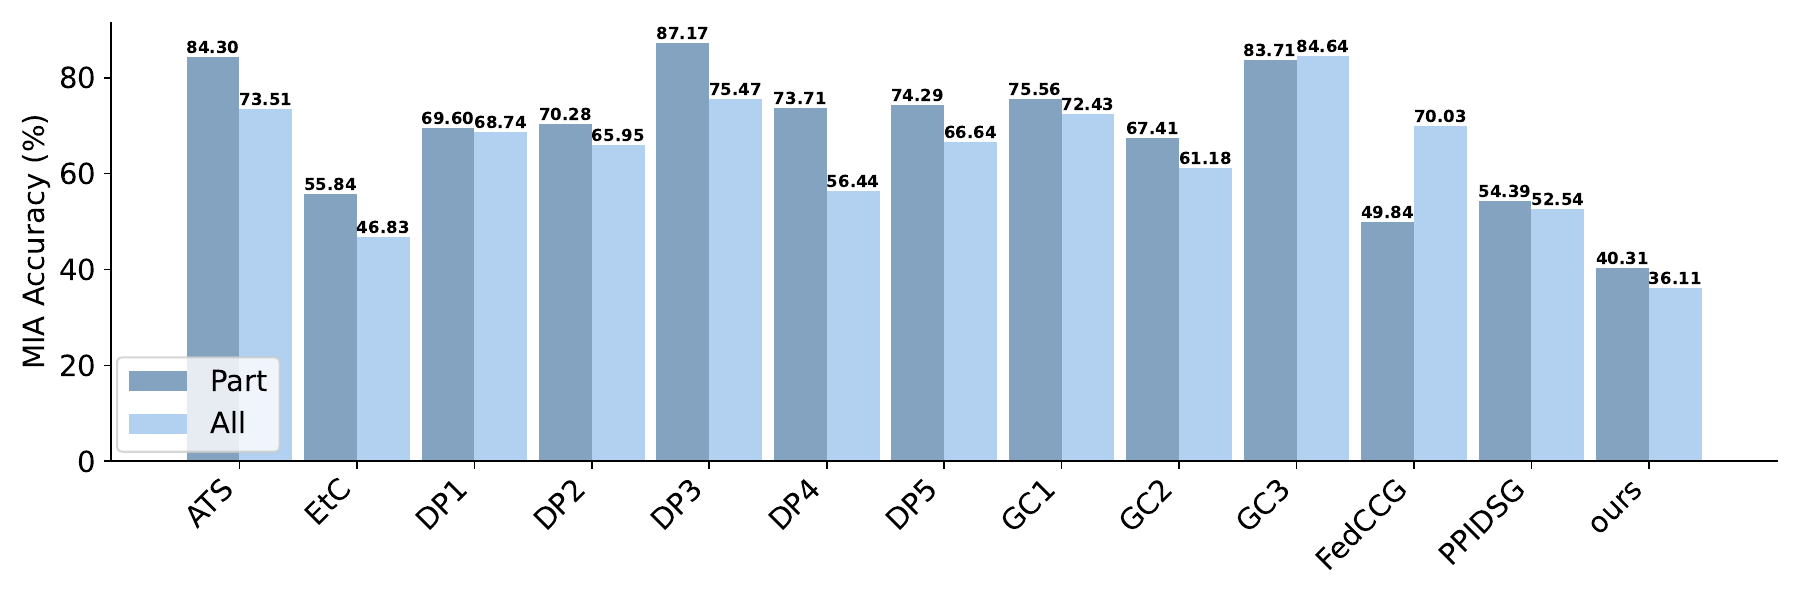}
    \caption{The MIA accuracy (\%) of different defense policies on CIFAR10 dataset (lower is better).}
   \label{fig:DEFENSE_MIA_CIFAR}
\end{figure}

\begin{figure}[H]
    \centering
    \includegraphics[width=8.75cm, height=4cm]{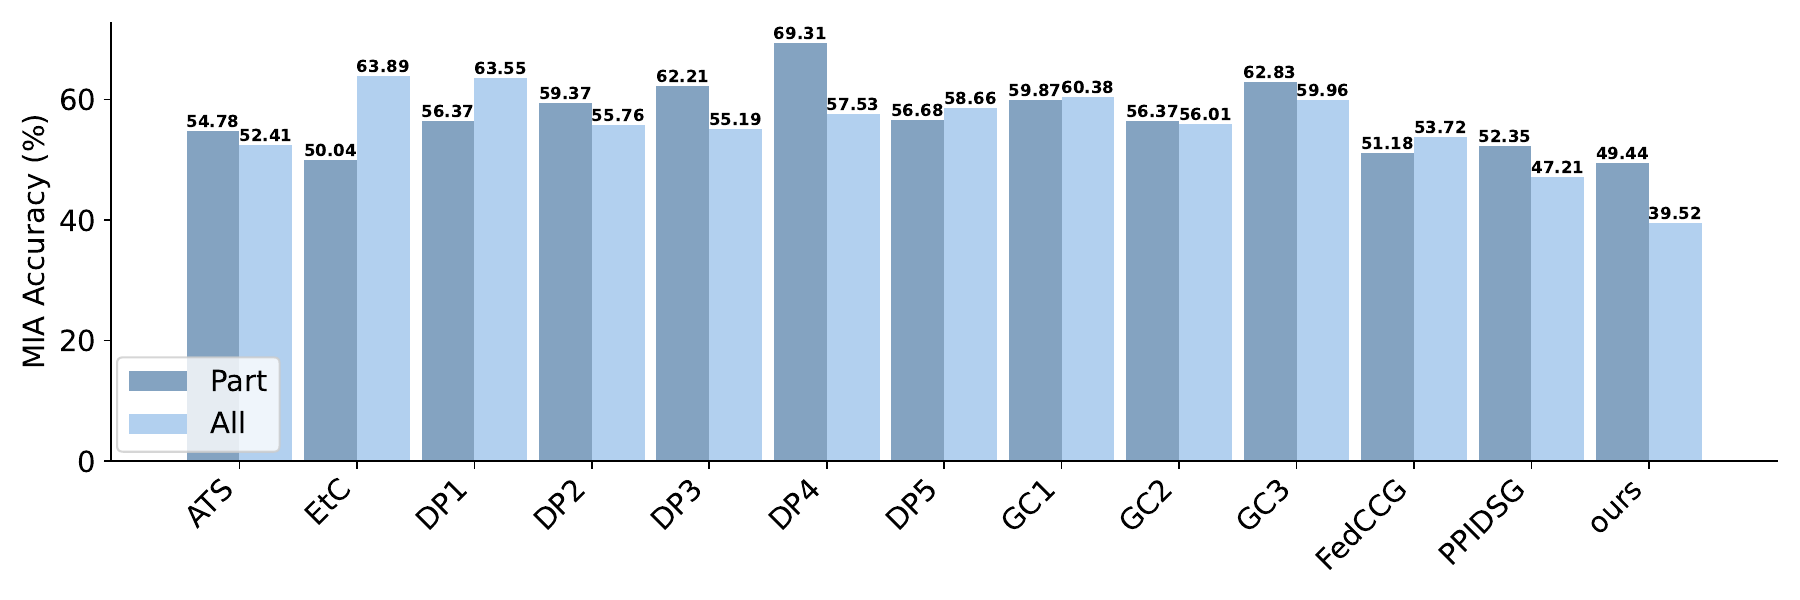}
    \caption{The MIA accuracy (\%) of different defense policies on SVHN dataset (lower is better).}
   \label{fig:DEFENSE_MIA_SVHN}
\end{figure}

\begin{table*}
    
    % \fontsize{7}{12}\selectfont
    \begin{tabular}{|c|c|c|c|c|c|c|c|}
        \hline
        \multicolumn{2}{|c|}{\textbf{Policy}} & \multicolumn{3}{c|}{\textbf{Part}} & \multicolumn{3}{c|}{\textbf{All}} \\
        \cline{3-8}
        \multicolumn{2}{|c|}{} & \textbf{Precision} & \textbf{Recall} & \textbf{F1-score} & \textbf{Precision} & \textbf{Recall} & \textbf{F1-score} \\
        \hline
        \multicolumn{2}{|c|}{ATS} & 0.50 (0.51) & 0.70 (0.31) & 0.59 (0.39) & 0.10 (0.90) & 0.80 (0.20) & 0.18 (0.33) \\\hline
        \multicolumn{2}{|c|}{EtC} & 0.50 (0.49) & 0.58 (0.41) & 0.53 (0.45) & 0.10 (0.90) & 0.39 (0.60) & 0.16 (0.72) \\\hline
        \multirow{5}{*}{DP} & $<5,10>$ & 0.54 (0.54) & 0.54 (0.54) & 0.54 (0.54) & 0.10 (0.90) & 0.45 (0.57) & 0.17 (0.70) \\
         & $<10,10>$ & 0.51 (0.51) & 0.61 (0.41) & 0.56 (0.45) & 0.10 (0.90) & 0.63 (0.38) & 0.18 (0.54) \\
         & $<20,10>$ & 0.51 (0.52) & 0.58 (0.45) & 0.54 (0.48) & 0.10 (0.90) & 0.64 (0.37) & 0.18 (0.53) \\
         & $<20,5>$ & 0.51 (0.52) & 0.61 (0.42) & 0.56 (0.46) & 0.10 (0.90) & 0.63 (0.39) & 0.18 (0.54) \\
         & $<20,20>$ & 0.52 (0.51) & 0.47 (0.56) & 0.49 (0.53) & 0.10 (0.90) & 0.71 (0.29) & 0.18 (0.44) \\\hline
        \multirow{3}{*}{GC} & p=10\% & 0.52 (0.52) & 0.49 (0.56) & 0.51 (0.54) & 0.11 (0.91) & 0.48 (0.56) & 0.18 (0.70) \\
         & p=20\% & 0.52 (0.53) & 0.59 (0.47) & 0.55 (0.50) & 0.10 (0.90) & 0.54 (0.48) & 0.17 (0.63) \\
         & p=40\% & 0.53 (0.53) & 0.52 (0.54) & 0.52 (0.53) & 0.10 (0.90) & 0.55 (0.47) & 0.17 (0.62) \\\hline
        \multicolumn{2}{|c|}{FedCG} & 0.51 (0.51) & 0.60 (0.41) & 0.55 (0.46) & 0.10 (0.90) & 0.79 (0.21) & 0.18 (0.34) \\\hline
        \multicolumn{2}{|c|}{PPIDSG} & 0.46 (0.42) & 0.59 (0.30) & 0.51 (0.35) & 0.09 (0.87) & 0.61 (0.30) & 0.15 (0.45) \\\hline
        \multicolumn{2}{|c|}{Ours}  
        & {0.47 (0.41)} & {0.78  (0.20)} & {0.58  (0.27)} & {0.10 (0.90)} & {0.80  (0.20)} & {0.18  (0.33)}\\
        \hline
    \end{tabular}
    \centering
     \caption{MIA performance comparison with different defenses policies under
Part and all settings for MNIST dataset (lower success rate is better). The numbers in brackets represent data from non-members, while those outside parentheses represent member data.}   
    \label{tab:MIA_MNIST}
\end{table*}
% \vspace{-0.5cm}
\begin{table*}
    \centering
   
    % \fontsize{7}{12}\selectfont
    \begin{tabular}{|c|c|c|c|c|c|c|c|}
        \hline
        \multicolumn{2}{|c|}{\textbf{Policy}} & \multicolumn{3}{c|}{\textbf{Part}} & \multicolumn{3}{c|}{\textbf{All}} \\
        \cline{3-8}
        \multicolumn{2}{|c|}{} & \textbf{Precision} & \textbf{Recall} &\textbf{F1-score} & \textbf{Precision} & \textbf{Recall} & \textbf{F1-score} \\
        \hline
        \multicolumn{2}{|c|}{ATS} & 0.55 (0.56) & 0.60 (0.50) & 0.57 (0.53) & 0.11 (0.91) & 0.58 (0.48) & 0.18 (0.63) \\\hline
        \multicolumn{2}{|c|}{EtC} & 0.52 (0.52) & 0.53 (0.50) & 0.53 (0.51) & 0.11 (0.91) & 0.49 (0.55) & 0.18 (0.68) \\\hline
        \multirow{5}{*}{DP} & $<5,10>$ & 0.58 (0.58) & 0.57 (0.59) & 0.58 (0.58) & 0.13 (0.92) & 0.54 (0.60) & 0.21 (0.73) \\
         & $<10,10>$ & 0.61 (0.58) & 0.52 (0.67) & 0.56 (0.62) & 0.14 (0.92) & 0.50 (0.67) & 0.22 (0.78) \\
         & $<20,10>$ & 0.61 (0.58) & 0.51 (0.67) & 0.55 (0.62) & 0.11 (0.91) & 0.64 (0.42) & 0.19 (0.58) \\
         & $<20,5>$ & 0.55 (0.55) & 0.58 (0.53) & 0.56 (0.54) & 0.12 (0.91) & 0.50 (0.58) & 0.19 (0.71) \\
         & $<20,20>$ & 0.58 (0.56) & 0.48 (0.66) & 0.52 (0.60) & 0.11 (0.92) & 0.64 (0.43) & 0.19 (0.59) \\\hline
        \multirow{3}{*}{GC} & p=10\% & 0.64 (0.61) & 0.58 (0.67) & 0.61 (0.64) & 0.16 (0.93) & 0.56 (0.67) & 0.25 (0.78) \\
         & p=20\% & 0.54 (0.57) & 0.69 (0.41) & 0.61 (0.48) & 0.13 (0.92) & 0.51 (0.61) & 0.20 (0.73) \\
         & p=40\% & 0.61 (0.67) & 0.75 (0.52) & 0.67 (0.58) & 0.13 (0.92) & 0.53 (0.61) & 0.21 (0.73) \\\hline
        \multicolumn{2}{|c|}{FedCG} & 0.50 (0.49) & 0.60 (0.30) & 0.54 (0.44) & 0.10 (0.90) & 0.40 (0.60) & 0.16 (0.72) \\\hline
        \multicolumn{2}{|c|}{PPIDSG} & 0.50 (0.50) & 0.40 (0.60) & 0.44 (0.55) & 0.12 (0.92) & 0.59 (0.50) & 0.19 (0.65) \\\hline
        \multicolumn{2}{|c|}{Ours} & 0.54 (0.55) & 0.51  (0.49) & 0.57  (0.52) &  {0.09 (0.87)} & 0.60  (0.30) &   {0.15 (0.45)} \\
        \hline
    \end{tabular}
    \caption{MIA performance comparison with different defenses policies under Part and all setting for FMNIST dataset (lower success rate is better). The numbers in brackets represent data from non-members, while those outside parentheses represent member data.}
    \label{tab:MIA_FMNIST}
\end{table*}

% \vspace{-0.5cm}
 \begin{table*}
    \centering
       
    % \fontsize{7}{12}\selectfont
    \begin{tabular}{|c|c|c|c|c|c|c|c|}
        \hline
        \multicolumn{2}{|c|}{\textbf{Policy}} & \multicolumn{3}{c|}{\textbf{Part}} & \multicolumn{3}{c|}{\textbf{All}} \\
        \cline{3-8}
        \multicolumn{2}{|c|}{} & \textbf{Precision} & \textbf{Recall} & \textbf{F1-score} & \textbf{Precision} & \textbf{Recall} & \textbf{F1-score} \\
        \hline
        \multicolumn{2}{|c|}{ATS} & 0.83 (0.86) & 0.87 (0.82) & 0.85 (0.84) & 0.24 (0.97) & 0.76 (0.73) & 0.37 (0.83) \\\hline
        \multicolumn{2}{|c|}{EtC} & 0.59 (0.54) & 0.38 (0.73) & 0.46 (0.62) & 0.10 (0.90) & 0.56 (0.46) & 0.17 (0.61) \\\hline
        \multirow{5}{*}{DP} & $<5,10>$ & 0.70 (0.69) & 0.69 (0.71) & 0.69 (0.70) & 0.19 (0.95) & 0.66 (0.69) & 0.30 (0.80) \\
         & $<10,10>$ & 0.71 (0.69) & 0.68 (0.73) & 0.70 (0.71) & 0.18 (0.95) & 0.68 (0.66) & 0.28 (0.78) \\
         & $<20,10>$ & 0.88 (0.87) & 0.87 (0.88) & 0.87 (0.87) & 0.25 (0.96) & 0.72 (0.76) & 0.37 (0.85) \\
         & $<20,5>$ & 0.74 (0.74) & 0.74 (0.74) & 0.74 (0.74) & 0.14 (0.93) & 0.64 (0.56) & 0.23 (0.70) \\
         & $<20,20>$ & 0.75 (0.73) & 0.72 (0.76) & 0.74 (0.75) & 0.19 (0.95) & 0.71 (0.66) & 0.30 (0.78) \\\hline
        \multirow{3}{*}{GC} & p=10\% & 0.78 (0.74) & 0.71 (0.80) & 0.75 (0.77) & 0.23 (0.96) & 0.75 (0.72) & 0.35 (0.82) \\
         & p=20\% & 0.69 (0.66) & 0.64 (0.71) & 0.66 (0.68) & 0.16 (0.94) & 0.65 (0.61) & 0.25 (0.74) \\
         & p=40\% & 0.85 (0.82) & 0.81 (0.86) & 0.83 (0.84) & 0.38 (0.98) & 0.82 (0.85) & 0.52 (0.91) \\\hline
        \multicolumn{2}{|c|}{FedCG} & 0.50 (0.50) & 0.60 (0.40) & 0.54 (0.44) & 0.11 (0.90) & 0.27 (0.75) & 0.15 (0.82) \\\hline
        \multicolumn{2}{|c|}{PPIDSG} & 0.57 (0.53) & 0.35 (0.74) & 0.43 (0.62) & 0.09 (0.89) & 0.40 (0.54) & 0.14 (0.67) \\\hline
        \multicolumn{2}{|c|}{Ours} &  {0.41 (0.40)} & 0.41  (0.40) &  {0.41 (0.40)} & 0.10 (0.90) & 0.62  (0.38) & 0.17  (0.54) \\
        \hline
    \end{tabular}
     \caption{MIA performance comparison with different defense policies under Part and all setting for CIFAR10 dataset (lower success rate is better). The numbers in brackets represent data from non-members, while those outside parentheses represent member data.}
    \label{tab:MIA_CIFAR10_supplymentry}
\end{table*}
\begin{table*}
    \centering
   
    % \fontsize{7}{12}\selectfont
    \begin{tabular}{|c|c|c|c|c|c|c|c|}
        \hline
        \multicolumn{2}{|c|}{\textbf{Policy}} & \multicolumn{3}{c|}{\textbf{Part}} & \multicolumn{3}{c|}{\textbf{All}} \\
        \cline{3-8}
        \multicolumn{2}{|c|}{} & \textbf{Precision} & \textbf{Recall} & \textbf{F1-score} & \textbf{Precision} & \textbf{Recall} &\textbf{ F1-score} \\
        \hline
        \multicolumn{2}{|c|}{ATS} & 0.54 (0.55) & 0.61 (0.48) & 0.58 (0.52) & 0.12 (0.92) & 0.61 (0.51) & 0.21 (0.66) \\\hline
        \multicolumn{2}{|c|}{EtC} & 0.50 (0.50) & 0.47 (0.54) & 0.48 (0.52) & 0.10 (0.90) & 0.32 (0.67) & 0.15 (0.77) \\\hline
        \multirow{5}{*}{DP} & $<5,10>$ & 0.57 (0.56) & 0.55 (0.58) & 0.56 (0.57) & 0.13 (0.91) & 0.45 (0.66) & 0.20 (0.76) \\
         & $<10,10>$ & 0.59 (0.60) & 0.64 (0.55) & 0.61 (0.57) & 0.11 (0.91) & 0.47 (0.57) & 0.18 (0.70) \\
         & $<20,10>$ & 0.60 (0.65) & 0.71 (0.53) & 0.65 (0.59) & 0.12 (0.92) & 0.56 (0.55) & 0.20 (0.69) \\
         & $<20,5>$ & 0.73 (0.67) & 0.61 (0.77) & 0.67 (0.71) & 0.12 (0.91) & 0.50 (0.58) & 0.19 (0.71) \\
         & $<20,20>$ & 0.57 (0.56) & 0.55 (0.59) & 0.56 (0.58) & 0.11 (0.91) & 0.46 (0.60) & 0.18 (0.72) \\\hline
        \multirow{3}{*}{GC} & p=10\% & 0.60 (0.60) & 0.61 (0.59) & 0.60 (0.59) & 0.13 (0.92) & 0.54 (0.61) & 0.21 (0.74) \\
         & p=20\% & 0.57 (0.56) & 0.54 (0.58) & 0.55 (0.57) & 0.12 (0.91) & 0.51 (0.57) & 0.19 (0.70) \\
         & p=40\% & 0.62 (0.63) & 0.65 (0.60) & 0.64 (0.62) & 0.16 (0.95) & 0.70 (0.58) & 0.25 (0.72) \\\hline
        \multicolumn{2}{|c|}{FedCG} & 0.51 (0.51) & 0.59 (0.43) & 0.55 (0.47) & 0.11 (0.91) & 0.49 (0.54) & 0.17 (0.68) \\\hline
        \multicolumn{2}{|c|}{PPIDSG} & 0.53 (0.52) & 0.41 (0.64) & 0.46 (0.57) & 0.09 (0.89) & 0.49 (0.47) & 0.16 (0.62) \\\hline
        \multicolumn{2}{|c|}{Ours} &  {0.50 (0.48)} & 0.83  (0.15) & 0.62  (0.23) & 0.09 (0.89) & 0.58  (0.37) & 0.16  (0.53) \\
        \hline
    \end{tabular}
     \caption{MIA performance comparison with different defenses policies under Part and all setting for SVHN dataset (lower success rate is better). The numbers in brackets represent data from non-members, while those outside parentheses represent member data.}
    \label{tab:MIA_SVHN}
\end{table*}

\clearpage
 {
    \small
    \bibliographystyle{ieeenat_fullname}
    \bibliography{ref}
}

% \section{Rationale}
% \label{sec:rationale}
% % 
% Having the supplementary compiled together with the main paper means that:
% % 
% \begin{itemize}
% \item The supplementary can back-reference sections of the main paper, for example, we can refer to \cref{sec:intro};
% \item The main paper can forward reference sub-sections within the supplementary explicitly (e.g. referring to a particular experiment); 
% \item When submitted to arXiv, the supplementary will already included at the end of the paper.
% \end{itemize}
% % 
% To split the supplementary pages from the main paper, you can use \href{https://support.apple.com/en-ca/guide/preview/prvw11793/mac#:~:text=Delete%20a%20page%20from%20a,or%20choose%20Edit%20%3E%20Delete).}{Preview (on macOS)}, \href{https://www.adobe.com/acrobat/how-to/delete-pages-from-pdf.html#:~:text=Choose%20%E2%80%9CTools%E2%80%9D%20%3E%20%E2%80%9COrganize,or%20pages%20from%20the%20file.}{Adobe Acrobat} (on all OSs), as well as \href{https://superuser.com/questions/517986/is-it-possible-to-delete-some-pages-of-a-pdf-document}{command line tools}.
